# Supplementary material for: No Time for Downtime: Understanding Post-Attack Behaviors by Customers of Managed DNS Providers
Source: arXiv:2205.12765 source file (2022-05-25)
Supplement: Supplementary file 2 [file appendix.tex]

% \appendices
% \section{Title of an Appendix}
% Appendix one text goes here.

% you can choose not to have a title for an appendix
% if you want by leaving the argument blank
% \section{}
% Appendix two text goes here. Without title


% use section* for acknowledgment
% \section*{Acknowledgment}


% The authors would like to thank...


% Can use something like this to put references on a page
% by themselves when using endfloat and the captionsoff option.
\ifCLASSOPTIONcaptionsoff
  \newpage
\fi



% trigger a \newpage just before the given reference
% number - used to balance the columns on the last page
% adjust value as needed - may need to be readjusted if
% the document is modified later
%\IEEEtriggeratref{8}
% The "triggered" command can be changed if desired:
%\IEEEtriggercmd{\enlargethispage{-5in}}
